# Supplementary material for: High-speed detection of 1550 nm single photons with superconducting nanowire detectors
Source: arXiv:2210.11644 ancillary file (2022-10-21)
Supplement: Supplementary file 1 [file PEACOQ_Supplemental_Document.pdf]

# High speed detection of telecommunications wavelength single photons with superconducting nanowire detectors

## Supplemental Information

### 1. DEVICE FABRICATION

The PEACQ array was fabricated on a silicon wafer. First a gold mirror (80 nm of Au with 1.5 nm Ti below and 2.5 nm Ti on top for adhesion) was patterned using optical lithography; the metals were deposited by electron beam deposition or DC sputtering and then lifted off. We sputtered a 240 nm layer of SiO<sub>2</sub> as a spacer layer, and then a  $\sim 7.5$  nm-thick niobium nitride (NbN) film was sputtered using DC sputtering and RF substrate bias. The sheet resistance of the film at room temperature was 735  $\Omega/\text{sq}$ , measured in the completed device after all processing. Bonding pads and coplanar waveguides were patterned using optical lithography, Ti/Nb (4.5/50 nm, sputtered) and Ti/Au/Ti (1.5/15/3.5 nm, electron beam deposition), and liftoff. Ion milling before deposition ensured good contact to the NbN. Electron beam lithography and plasma etching with fluorine chemistry were used to define the nanowires and microstrip transmission lines. Finally, a 4-layer distributed bragg reflector of alternating SiO<sub>2</sub> and TiO<sub>2</sub> was deposited using sputtering. From the nanowire layer up, the dimensions were 254 nm SiO<sub>2</sub>, 175 nm TiO<sub>2</sub>, 275 nm SiO<sub>2</sub>, 139 nm TiO<sub>2</sub>. The film was monitored using a normal incidence spectral reflectance tool [1] at various times in the deposition to ensure that reflectance at 1550 nm was minimized. The device was then released from the wafer using deep reactive ion etching (DRIE) in two steps: first the oxide layers, then the silicon wafer.

### 2. CROSS-TALK

Cross-talk between nanowires in an array can be either electrical or thermal in nature. Electrical cross-talk can occur between the wires themselves, or later in the circuit, such as in the cables or TDC. We observed cross-talk between neighboring wires for some wires in the array. Based on the timescale and bias current dependence of the cross-talk, we believe the cross-talk is thermal in nature.

Figure S1 shows the distribution of successive counts on two neighboring wires as a function of delay. The analysis is done for two wires, one of which experiences significantly more cross-talk. Time-tags were recorded for all channels while measuring an attenuated continuous-wave laser. The recorded tags were then searched for instances where wire  $m$  measured a count followed by wire  $n$  measuring a count, where  $m$  and  $n$  are two adjacent wires. The probability of these two counts being offset by a delay  $t'$  is described by the conditional probability that once wire  $m$  detects a count at  $t = 0$ , wire  $n$  then detects a count within  $dt$  of  $t'$ ,  $P_{n,m}(t') \equiv P(c_n = 1, t' < t \leq t' + dt | c_m = 1, t = 0)$ , where  $c_k$  is the number of counts on wire  $k$ . Since  $c_n$  and  $c_m$  are described by Poisson statistics,  $P_{n,m}(t') = e^{-\Gamma_m t'} \times e^{-\Gamma_n t'} \times \Gamma_n dt e^{-\Gamma_n dt}$ , where the first two terms describe the probability that neither wire  $m$  nor  $n$  detects a count between  $t = 0$  and  $t = t'$ , and the last term describes the probability of wire  $n$  detecting a count during  $dt$ . This expression is plotted in Fig. S1 for each combination of wires as a solid black curve. It can be seen that in the absence of cross-talk, this curve fits the data well. Wire 8 shows evidence of cross-talk as there are more counts on wire 8 than predicted by Poissonian statistics approximately 6 ns after either wire 7 or 9 detects a count. The number of cross-talk counts can be estimated by measuring the area of the unscaled histogram above the baseline level of counts. Note that the figure is only showing events where counts on wire  $m$  were immediately preceded by counts on wires  $m - 1$  or  $m + 1$ , and not all counts on wire  $m$ . The size of the peak at 6 ns is therefore not a visual representation of the fraction of counts due to cross-talk.

When biasing the nanowires at 95% of their switching current, 13/32 wires had detectable cross-talk counts at a 6 ns delay, with wire 8 having the highest fraction. Of a total of 25 million tags measured across the array, 0.4% were attributed to cross-talk counts. All wires showing

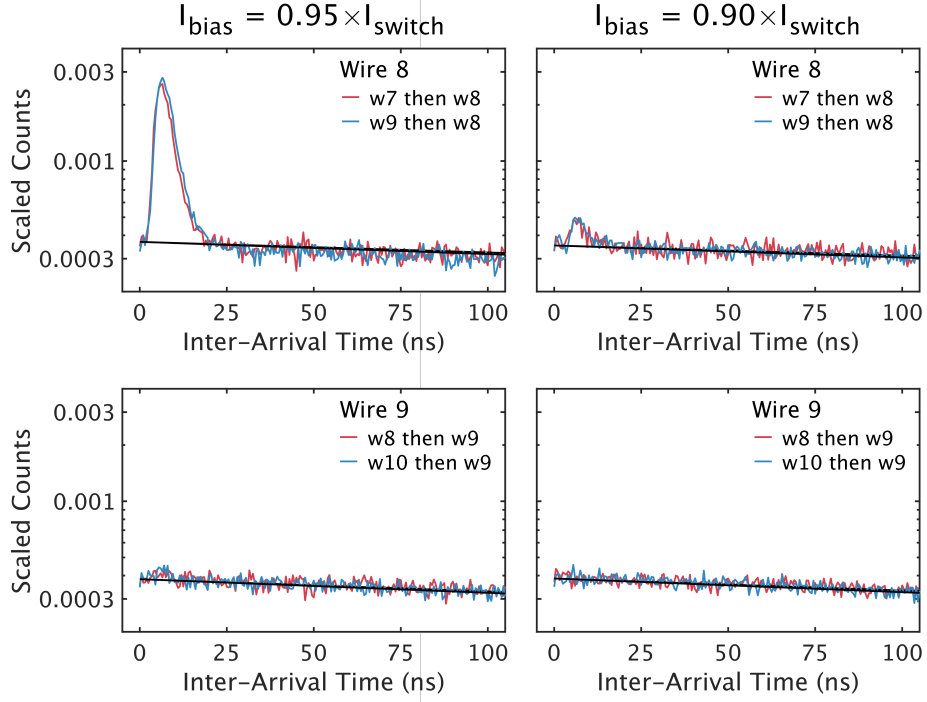

**Fig. S1.** Cross-talk in nanowires 8 and 9 when biased at  $I_{\text{bias}} = 0.95 \times I_{\text{switch}}$  (left side) and  $I_{\text{bias}} = 0.90 \times I_{\text{switch}}$  (right side). Red (blue) curve shows a scaled histogram of events where the wire to the left (right) detected a count, followed by the wire in question detecting a count, as a function of delay time between the two counts. Black curve is a theoretical curve describing the probability of this sequence of events given a Poisson-distributed input source. Peak at 6 ns shows evidence of cross-talk between wire 8 and its neighbors.

cross-talk were symmetric with respect to their nearest neighbors – if they saw cross-talk from one neighbor, they also saw cross-talk from the other neighbor.

When biasing the nanowires at 90% of their switching current, 5/32 wires showed cross-talk, and the fraction of total counts attributed to cross-talk was  $< 0.02\%$ . This bias current dependence is expected for thermal cross-talk between nanowires [2]. Operating at a lower bias current is an effective way to eliminate the observed cross-talk. Alternately, an array with larger pitch or narrower nanowires which have lower hotspot energy could be used.

### 3. OPTICAL STACK DESIGN

Rigorous coupled wave analysis (RCWA) was used to simulate the optical stack. Figure S2a shows a schematic of the optical stack. Figure S2b shows a RCWA simulation of absorption in the nanowire layer. The simulation assumes a plane wave at normal incidence to the device surface. The nanowire layer is modelled as an infinite grating, and all other layers are assumed to be homogeneous. Layer thicknesses are as described in the Device Fabrication section.

The simulation gives insight into the approximate bandwidth and polarization-dependence of the design. The stack was chosen to maximize the average absorption for the two orthogonal polarizations as a way to create a polarization-insensitive detector. At 1550 nm, we measured a spread of  $< 1\%$  in detection efficiency as a function of polarization, within our measurement error. In the simulation, the equal absorption efficiency for the two polarizations occurs at 1540 nm, indicating that simulated stack differs somewhat from the real detector. One source of error in the simulation is uncertainty in the complex refractive indices of the materials. We used values for  $n$  and  $k$  measured at room temperature. Additional sources of error are uncertainty in the thickness of the superconductor, to which the simulation is quite sensitive, and modelling an optical fiber mode with a numerical aperture of 0.14 as a plane wave.

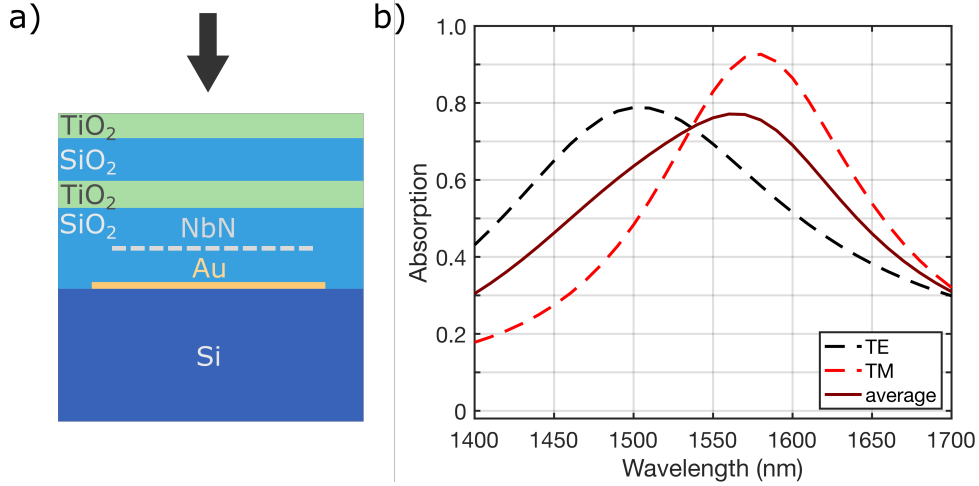

**Fig. S2.** Optical Stack. a) Diagram of optical stack. Arrow shows direction of light. b) Simulation of absorption in PEACQ nanowire layer. Dashed black curve shows absorption of light polarized parallel to the long axis of the nanowires (TE), dashed red line shows absorption of light perpendicular to the nanowires (TM). Solid dark red line is an average of the two curves.

#### 4. MAXIMUM COUNT RATE

Figure S3 shows the effect of various parameters on the maximum count rate of the array. Figure S3a shows that a small change in bias current, which can be used to decrease cross-talk between the wires, did not significantly affect the MCR. On the other hand, increasing the threshold level of the TDC from 25% to 45% of the pulse amplitude did have a noticeable effect on array MCR. This is because at high count rates, detection events are likely to occur while the nanowires are still recovering from the previous detection, leading to smaller pulses that will be missed by a larger threshold. Note that when the threshold was set to 25% of the pulse amplitudes on each channel, the trigger level on the channel corresponding to nanowire 14 was set to 33% to avoid triggering on the larger amplifier noise seen on that channel.

Figure S3b shows the theoretical effect on the timescale of post-detection efficiency recovery of either doubling the detection efficiency plateau  $I_{\text{switch}} - (I_{\text{detect}} + \sigma)$  by increasing the bias current from 13.3  $\mu\text{A}$  to 16  $\mu\text{A}$  or halving the reset time  $\tau_{\text{reset}} = \frac{L_R^k}{R_L}$ . The dead time of an individual nanowire decreases in both scenarios. Either increasing the plateau or decreasing the reset time are effective strategies in increasing the MCR of individual nanowires.

Figure S3c shows the effect of changing the array pitch on the array efficiency and MCR. We define the efficiency of the PEACQ array as a function of array count rate as  $\eta_{\text{array}}(\text{CR}_{\text{array}}; p)$ :

$$\eta_{\text{array}}(\text{CR}_{\text{array}}; p) = \frac{1}{\text{CR}_{\text{input}}} \sum_i^{32} \text{CR}_i \times \eta_R(\text{CR}), \quad (\text{S1})$$

where  $\text{CR}_{\text{input}}$  is the photon rate incident on the array,  $p$  is the pitch of the array,  $\text{CR}_i = \eta_{o,i}(p) \times \text{CR}_{\text{input}}$  is the count rate expected for each nanowire in the absence of count rate saturation and  $\eta_{o,i}(p)$  is the fraction of photons detected by each wire at low count rates (as in Fig. 2);  $\eta_R(\text{CR})$  is the relative efficiency on a nanowire as a function of count rate, describing saturation effects (blue curve in 3a). We approximate  $\eta_R(\text{CR})$  as being the same for all nanowires, taking an average MCR value. For this calculation, it is assumed that the fraction of photons absorbed by the array depends only on the fraction of the optical mode covered by the array:  $\eta_{o,i}(p) = \int_{p(i-16.5)-p/2}^{p(i-16.5)+p/2} f(x)$ , and  $f(x)$  is the normalized distribution of the SMF-28 optical mode (as in Fig. 2). This calculation ignores the fact that a lower pitch (higher fill factor) leads to more absorption in a grating comprised of absorbing nanowires separated by non-absorbing dielectric. This latter effect can be compensated to an extent by changing the optical stack, so it is reasonable to ignore it in order to more simply illustrate the trade-offs between efficiency and MCR in the array.

Figure S3c shows  $\eta_{\text{array}}(\text{CR}_{\text{array}}; p)$  for three array pitches, with the central value  $p = 400$  nm

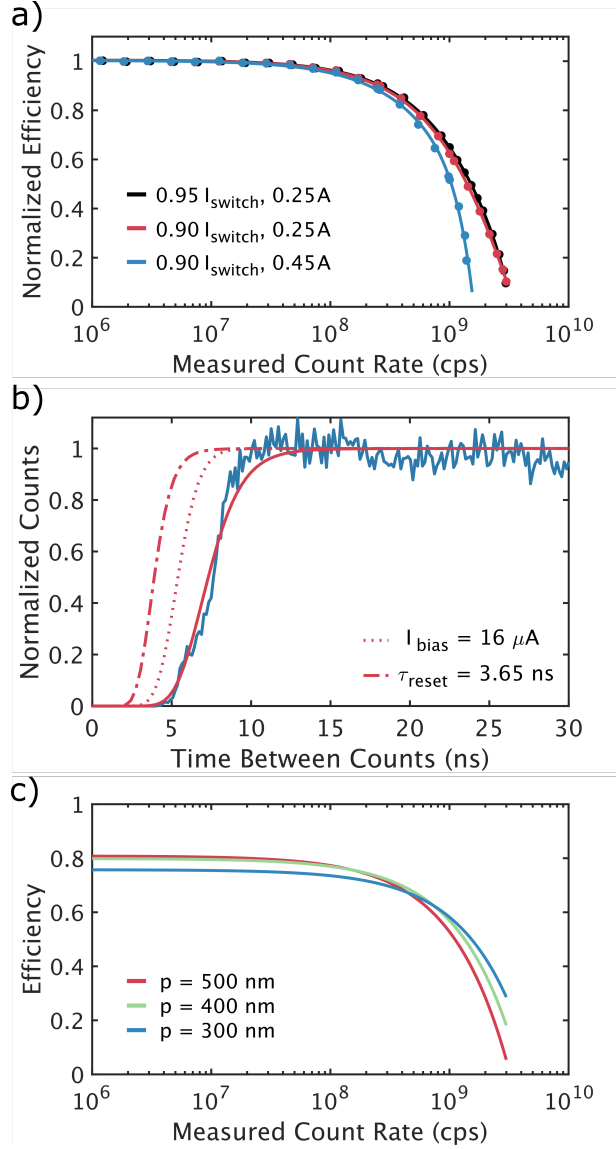

**Fig. S3.** The effect of TDC threshold, bias current, and array pitch on MCR. a) Normalized array efficiency versus count rate when using different bias currents, expressed as a fraction of the switching current, and different TDC threshold levels, expressed as a fraction of pulse amplitude  $A$ . Black curve is the same as in Figure 3a. b) Theoretical efficiency versus time since the last detection for one wire. Solid curves are the same as in Figure 3b. Dotted line shows the predicted efficiency curve for a wire with a plateau  $I_{\text{switch}} - (I_{\text{detect}} + \sigma)$  that is twice as long (assuming the nanowire is biased close to its critical current,  $I_{\text{bias}} \approx I_{\text{switch}}$ ), and otherwise identical parameters. Dot-dashed line shows same for a wire half the reset time but otherwise identical parameters. c) Theoretical calculations of efficiency versus count rate for similar arrays with different pitch.

being the same as in the device measured. A larger pitch leads to a slightly higher efficiency since the array covers more of the tails of the optical mode. However, the center of the optical mode where photons are incident at a higher rate is now covered by fewer nanowires, so they will saturate faster, leading to a decreased array MCR. The converse is true for the lower pitch.

## 5. JITTER

### A. Additional Jitter Measurements

Figure S4 shows additional timing jitter data supporting the main text. Figure S4a shows the timing jitter histogram measured for nanowire 1 using a 10 MHz pulsed laser and a Becker-Hickl TCSPC card, which uses a constant fraction discriminator and has a timing resolution of 1.1 ps. The jitter measurement of 16.8 ps FWHM/44.7 ps FW1%M is slightly lower than measured with the Swabian time card and places an upper bound on intrinsic nanowire jitter. Figure S4b shows the low-count-rate jitter as measured with the 128-channel TDC from Dotfast Consulting (black circles and blue curve, 84.3 ps FWHM/202.3 ps FW1%M) and the estimated low count rate jitter for an improved readout setup, as estimated from jitter measurements in Setup B (green curves, 21 ps FWHM/66 ps FW1%M with a 2<sup>nd</sup> order correction). Time-walk correction is not necessary at low count array count rates, as seen by the high degree of overlap between the corrected and raw curves. Figure S4c shows the estimated jitter at an array count rate of 1 Gcps with and without timing jitter correction. With a 2<sup>nd</sup> order correction, the jitter is 46 ps FWHM/244 ps FW1%M. Figure S4 summarizes the estimated time-walk-corrected jitter at several array count rates. It can be seen that a second order correction is effective at reducing time-walk-induced jitter at array count rates up to 250 Mcps, where the jitter histogram after 2<sup>nd</sup> order correction is very similar to the low count rate histogram.

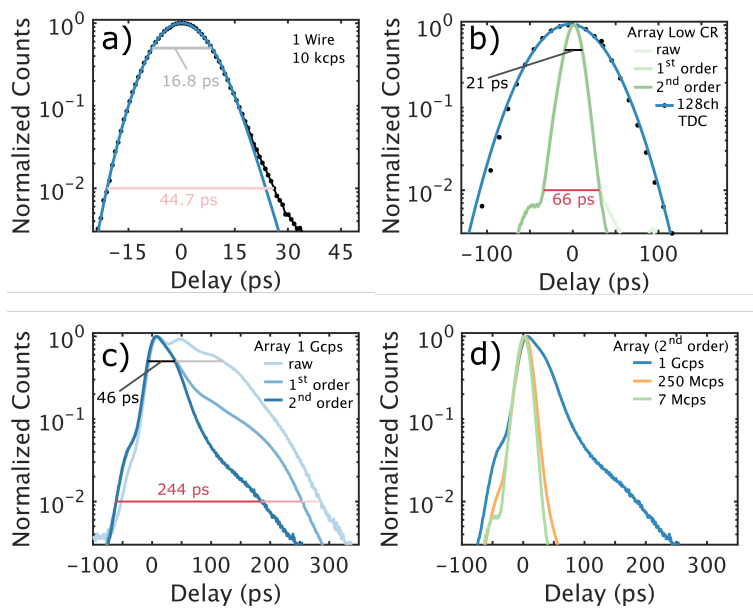

**Fig. S4.** Additional timing jitter data. Black and red horizontal lines show FWHM and FW1%M as in Fig. 4c. a) Black circles show the jitter histogram for nanowire 1 measured with Setup B a Becker-Hickl time card. Blue line is a fit to an exponentially modified Gaussian. b) Array jitter at low count rates. Black circles show the array jitter as measured with the 128-channel TDC (Setup A) and blue line is an exponentially modified Gaussian fit. Green curves show the array jitter at a low count rates (7 Mcps across the whole array) as predicted from the single nanowire jitter measured in Setup B. c) Predicted array jitter for an count rate of 1 Gcps. Darker shades indicate time-walk correction. d) Predicted timing jitter at different array count rates with 2<sup>nd</sup> order correction. Data is the same as b), c) and Fig. 4b.

Two nanowires, 1 and 16, were characterized in Setup B. The low-count rate timing jitter for wire 16 was 15.6 ps FWHM/44.2 ps FW1%M as measured with the Becker-Hickl time card. The time-walk correction analysis was also performed using nanowire 16, and the total array jitter estimates were uniformly lower than for the same analysis using nanowire 1. The array jitter estimates based on jitter measurements of nanowire 1 were the ones presented in Figures 4 and S4, being the more conservative estimate.

All jitter measurements in Figures 4 and S4 were taken with wires biased at 95% of their switching current. The estimate of array jitter with time-walk correction was also performed

with nanowire 1 biased at 90% of its switching current, and the array jitter estimates were found to differ by up to 10%. At low array count rates, the array jitter estimate increased slightly (22 ps FWHM/70 ps FW1%M at 7 Mcps with 2<sup>nd</sup> order correction), but at higher array count rates, the estimated jitter actually decreased (43 ps FWHM/222 ps FW1%M at 1 Gcps with 2<sup>nd</sup> order correction). This might be because when nanowires are biased at a lower current, the pulses exhibiting the most to time-walk-induced jitter are so small as to be below the threshold level, such that they are not counted. This could lead to a lower jitter at higher count rates, where these small pulses are most common and contribute to a long tail in jitter histograms.

## B. First Order Time Walk Correction

The jitter correction technique shown in this article employs and builds on the techniques first introduced in Reference [3].

At high count rates, SNSPD pulses may be undersized or distorted due effects of the amplification chain or intrinsic features of the nanowire reset process. These variations in pulse shape and height cause the constant trigger threshold of the TDC to ‘walk’ along the rising edge of the SNSPD pulse by varying amounts. Due to this, the timing measurements become corrupted by unmanaged delays. However, the delay observed for any one SNSPD pulse is correlated with the time since the previous SNSPD pulse, as this delay time can carry information about the reset state of the nanowire or the overshoot/ringing state of the amplifier chain.

Reference [3] introduces a calibration process which produces a lookup table. It is used during real-time data collection or in post-processing to correct pulse time measurements based on preceding inter-pulse time. The calibration process used to create the lookup table relies on measuring the arrival time of distorted high count rate pulses with respect to the highly regular timing of a mode locked laser.

A 1-GHz repetition rate 1550 nm mode locked laser was used (Pritel UOC) for calibration. The repetition rate of the laser determines the resolution of the resulting calibration curve. The 1 GHz repetition rate was chosen so that uncorrected jitter even at the highest count rates (approaching 400 ps at the FW1%M), was smaller than the laser period. Then, each time tag could be matched to the timing of the original optical pulse. A dataset with a count rate of 20 MCounts/s was used for calibration. At this rate, there is a good balance of statistics available for  $t'$  ranging between 5 and 150 ns.

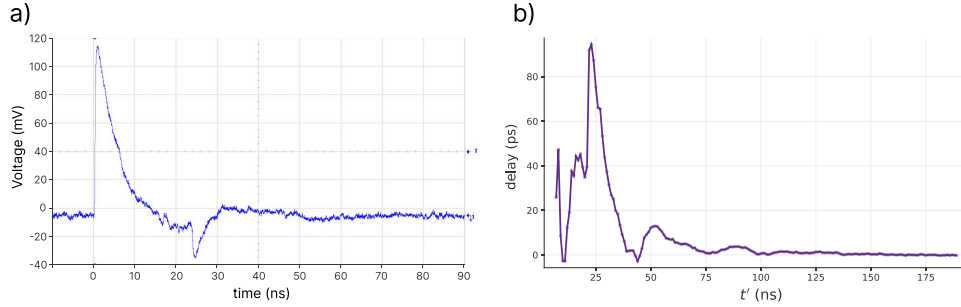

**Fig. S5.** a) The RF pulse of one of the PEACOQ nanowires. The effect of an impedance mismatch reflection is visible at 25 ns. b) The delay vs  $t'$  curve for wire 1 of the PEACOQ. The peak at 25 ns lines up in time with the RF reflection visible in (a), and works to correct for the time-walk delays it causes.

The calibration process for the PEACOQ showed that high-rate pulse distortions are primarily due to amplifier effects and the overlap of RF pulses with the overshoot or ringing effects of previous RF pulses. This is because the nanowire design and fabrication of the PEACOQ seeks to minimize the intrinsic reset time of the nanowire. The time it takes for bias current to re-saturate in the device is generally faster than the time for all amplifier effects to disappear following a previous RF pulse. S5b is the delay vs.  $t'$  curve derived from the calibration process. Unlike Figure 3a in Reference [3], the delay vs.  $t'$  curve for the PEACOQ shows features that are closely related to the falling edge of the RF pulse (S5a). Future implementations of the PEACOQ will optimize the amplification chain for minimal RF reflections.

Though the calibration was conducted with attenuated laser pulses derived from a 1-GHz laser, there is no requirement that the calibration only be used in an application that's based on

the same repetition rate. As interpolation between points on the delay vs.  $t'$  vslookup curve is possible, delay corrections for arbitrary  $t'$  measurements may be found.

### C. Second Order Time Walk Correction

The 2<sup>nd</sup> order time-walk correction is a new technique that builds on the methods from Reference [3] and is demonstrated here for the first time. The intrinsic reset time of the PEACQ nanowires is considerably shorter than the time it takes an RF pulse to return to a steady zero voltage. So multiple pulses can arrive in the time it takes one RF pulse to fully decay as seen by the timing electronics. Therefore, a given RF pulse can be level shifted not only by the presence of a previous pulse a few nanoseconds earlier, but even by the presence of two previous pulses. The calibration and correction process from Reference [3] was extended to correct a given pulse timing measurement based on two inter-pulse time measurements  $t'$  and  $t''$  as shown in S6a. The calibration process uses the same mode-locked laser derived pulse train as the 1<sup>st</sup> order calibration. For each  $t'$  there is a full range of possible  $t''$  times and vice versa, so the result of calibration becomes a 2D grid of delay corrections indexed by  $t'$  and  $t''$ .  $t'$  is always less than  $t''$  for the parameterization chosen, where both are measured from the latest or 'current' time tag (S6a). Therefore, the space of valid measurements is triangular as shown in S6b.

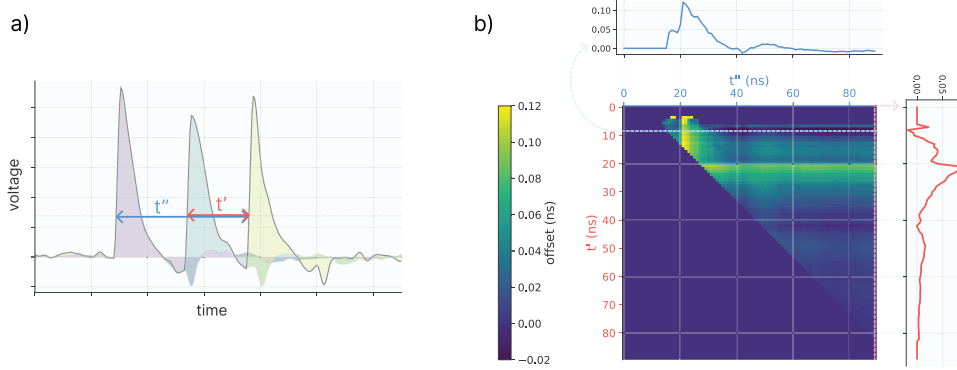

**Fig. S6.** a) A diagram showing how RF pulse waveforms can interfere additively, and how  $t'$  and  $t''$  are parameterized. For illustrative purposes only. b) The result of 2<sup>nd</sup> order calibration, a grid of delay measurements indexed by  $t'$  and  $t''$ . The blue/red slices and corresponding graphs show how the effect of varying  $t''$  for a given  $t'$  is similar to varying  $t'$  for a given  $t''$ .

In the limit of large  $t''$ , a slice of the calibration grid bears close resemblance to the  $t'$  vs delay curve used for 1D calibration and correction (S5b). Like in the 1D correction method, a delay correction can be found during real-time acquisition and processing by interpolating on a lookup table. Only now, the lookup table has an extra dependent variable  $t''$ , and the interpolation is two dimensional.

Proper handling of inter-pulse arrival measurements that fall outside the 2D grid is necessary for good correction performance. When both  $t'$  and  $t''$  fall outside the 2D grid, no correction is applied. When  $t''$  falls outside the grid but  $t'$  does not, a 1<sup>st</sup> order correction is applied to determine what delay must be subtracted to the current tag to correct its distortion. When both  $t''$  and  $t'$  fall within the 2d grid, a full 2d spline interpolation on the grid in S6b is applied to find the necessary delay correction.

The codebase supporting our findings with the 1<sup>st</sup> order and 2<sup>nd</sup> order correction is available at <https://github.com/sansseriff/SNSPD-time-walk-and-jitter-correction>

### REFERENCES

1. Filmetrics F40-UVX, KLA Corporation.
2. J. P. Allmaras, E. E. Wollman, A. D. Beyer, R. M. Briggs, B. A. Korzh, B. Bumble, and M. D. Shaw, "Demonstration of a thermally coupled row-column snspsd imaging array," *Nano Lett.* **20**, 2163–2168 (2020). PMID: 32091221.
3. A. Mueller, E. E. Wollman, B. Korzh, A. D. Beyer, L. Narvaez, R. Rogalin, M. Spiropulu, and M. D. Shaw, "Time-walk and jitter correction in snspsds at high count rates," *arXiv:2210.01271* (2022).
